# Supplementary material for: Mimicking the earth core conditions with ultrafast laser materials interaction
Source: arXiv:2602.22460 source file (2026-02-25)
Supplement: Supplementary file 1 [file Supplemental.tex]

\documentclass[pdflatex,sn-nature]{sn-jnl}

\usepackage{graphicx}
\usepackage{amsmath,amssymb}
\usepackage{booktabs}
\usepackage{siunitx}
\setlength{\oddsidemargin}{\evensidemargin}
\setlength{\parskip}{6pt}
% Remove all section numbering
\setcounter{secnumdepth}{0}

\begin{document}
\title[Article Title]{Mimicking the earth's core conditions with ultrafast laser materials interaction - Supplemental Information}
\maketitle

\end{document}
